# Supplementary material for: Designing clinical trials for the comparison of single and multiple quantiles with right-censored data
Source: arXiv:2505.03234 source file (2026-03-09)
Supplement: Supplementary file 1 [file supp_materials.pdf]

---

# Supplemental material: Univariate and multivariate tests of equality of quantiles with right-censored data

## Contents

|          |                                                 |          |
|----------|-------------------------------------------------|----------|
| <b>1</b> | <b>Proofs and Technical details</b>             | <b>2</b> |
| 1.1      | Univariate test . . . . .                       | 2        |
| 1.2      | Multivariate test . . . . .                     | 4        |
| <b>2</b> | <b>Details on the estimation of the density</b> | <b>6</b> |
| 2.1      | Resampling procedure . . . . .                  | 6        |
| 2.2      | Kernel density estimation . . . . .             | 10       |

# 1 Proofs and Technical details

## 1.1 Univariate test

In this section, we present the proofs for the results in Section 2.1 of the main document, for the univariate test. We first recall the expression of the statistical test in the univariate case.

$$\mathcal{T}_n = \sqrt{n} \frac{\hat{F}_1^{-1}(p) - \hat{F}_2^{-1}(p)}{\hat{\sigma}_{\mathcal{H}_0}}, \text{ with}$$

$$\hat{\sigma}_{\mathcal{H}_0}^2 = (1-p)^2 \left( \frac{\hat{\phi}_1}{\hat{\mu}_1 \hat{f}_1(\hat{F}_1^{-1}(p))^2} + \frac{\hat{\phi}_2}{\hat{\mu}_2 \hat{f}_2(\hat{F}_2^{-1}(p))^2} \right).$$

**Result 1.** Under  $\mathcal{H}_0 : F_1^{-1}(p) = F_2^{-1}(p)$ ,  $\mathcal{T}_n \xrightarrow{d} \mathcal{N}(0, 1)$  as  $n \rightarrow \infty$

**Proof.** From Lemma 1 from Kosorok<sup>1</sup>, for  $k = 1, 2$ ,

$$\hat{F}_k^{-1}(p) - F_k^{-1}(p) = \frac{\hat{F}_k(F_k^{-1}(p)) - p}{f_k(F_k^{-1}(p))} + o_p\left(\frac{1}{\sqrt{n_k}}\right)$$

It follows from Theorem 6.3.1 from Fleming and Harrington<sup>2</sup> that:

$$\sqrt{n_k} \left( \frac{\hat{F}_k(F_k^{-1}(p)) - p}{f_k(F_k^{-1}(p))} \right) \xrightarrow{d} \mathcal{N}\left(0, (1-p)^2 \frac{\phi_k}{f_k(F_k^{-1}(p))}\right), \text{ with}$$

$$\phi_k = \int_0^{F_k^{-1}(p)} \frac{d\Lambda_k(x)}{H_k(x)}.$$

Under  $\mathcal{H}_0$ , from the independence between treatment groups, as  $n \rightarrow \infty$ , we have that

$$\sqrt{n} \left[ \frac{\hat{F}_1(F_1^{-1}(p)) - p}{f_1(F_1^{-1}(p))} - \frac{\hat{F}_2(F_2^{-1}(p)) - p}{f_2(F_2^{-1}(p))} \right] \xrightarrow{d} \mathcal{N}\left(0, (1-p)^2 \left[ \frac{\phi_1}{\mu_1 f_1(F_1^{-1}(p))^2} + \frac{\phi_2}{\mu_2 f_2(F_2^{-1}(p))^2} \right]\right)$$

Then,  $\hat{\sigma}_{\mathcal{H}_0} \rightarrow \sigma_{\mathcal{H}_0}$  as  $n \rightarrow \infty$  from the consistency of Greenwood's estimator of the Kaplan-Meier variance, the consistency of the density estimators and the consistency of  $\hat{\mu}_k$ ,  $k = 1, 2$ . Finally under  $\mathcal{H}_0$ , we have the decomposition

$$\hat{F}_1^{-1}(p) - \hat{F}_2^{-1}(p) = \hat{F}_1^{-1}(p) - F_1^{-1}(p) - (\hat{F}_2^{-1}(p) - F_2^{-1}(p)),$$

which concludes the proof.

**Result 2.** Under  $\mathcal{H}_1 : F_1^{-1}(p) - F_2^{-1}(p) = \Delta$ ,  $\mathcal{T}_n - \sqrt{n} \frac{\Delta}{\hat{\sigma}_{\mathcal{H}_0}} \xrightarrow{d} \mathcal{N}(0, 1)$  as  $n \rightarrow \infty$

**Proof.** Under  $\mathcal{H}_1$ ,

$$\sqrt{n}(\hat{F}_1^{-1}(p) - \hat{F}_2^{-1}(p)) = \sqrt{n}(\hat{F}_1^{-1}(p) - F_1^{-1}(p)) - \sqrt{n}(\hat{F}_2^{-1}(p) - F_2^{-1}(p)) + \sqrt{n}\Delta.$$

We denote

$$Z_n = \sqrt{n}(\hat{F}_1^{-1}(p) - F_1^{-1}(p)) - \sqrt{n}(\hat{F}_2^{-1}(p) - F_2^{-1}(p)).$$

Then, from Lemma 1 from Kosorok<sup>1</sup>,

$$Z_n = \sqrt{n} \left( \frac{\hat{F}_1(F_1^{-1}(p)) - p}{f_1(F_1^{-1}(p))} \right) - \sqrt{n} \left( \frac{\hat{F}_2(F_2^{-1}(p)) - p}{f_2(F_2^{-1}(p))} \right) + o_p \left( \frac{1}{\sqrt{n}} \right).$$

It follows, for  $n \rightarrow \infty$ :

$$Z_n \xrightarrow{d} \mathcal{N} \left( 0, \frac{(1-p)^2 \phi_1}{\mu_1 f_1(F_1^{-1}(p))^2} + \frac{(1-p)^2 \phi_2}{\mu_2 f_2(F_2^{-1}(p))^2} \right)$$

From the consistency of  $\hat{\sigma}_{\mathcal{H}_0}$ , we therefore have  $Z_n/\hat{\sigma}_{\mathcal{H}_0} \xrightarrow{d} \mathcal{N}(0, 1)$ , which gives the desired result using the relation

$$\mathcal{T}_n = Z_n/\hat{\sigma}_{\mathcal{H}_0} + \sqrt{n}\Delta/\hat{\sigma}_{\mathcal{H}_0}.$$

**Result 3.** We have the following asymptotic formula for the power of the test of level  $\alpha$ :

$$1 - \beta \approx 1 - \Phi \left( q_{1-\alpha/2} - \frac{\sqrt{n}}{\hat{\sigma}_{\mathcal{H}_0}} \Delta \right) + \Phi \left( -q_{1-\alpha/2} - \frac{\sqrt{n}}{\hat{\sigma}_{\mathcal{H}_0}} \Delta \right)$$

where  $\Phi$  is the cumulative distribution function of the standard normal variable and  $q_{1-\alpha/2}$  is the quantile of level  $1 - \alpha/2$  of the standard normal distribution.

**Proof.** Using the derived expression for the test statistic and denoting as  $q_{1-\frac{\alpha}{2}}$  the quantile of order  $1 - \frac{\alpha}{2}$  of the standard normal distribution,

$$\begin{aligned} 1 - \beta &= P_{\mathcal{H}_1}(|\mathcal{T}_n| > q_{1-\frac{\alpha}{2}}) \\ &= P_{\mathcal{H}_1} \left( \sqrt{n} \left| \frac{\hat{F}_1^{-1}(p) - \hat{F}_2^{-1}(p)}{\hat{\sigma}_{\mathcal{H}_0}} \right| > q_{1-\frac{\alpha}{2}} \right) \\ &= P_{\mathcal{H}_1} \left( \sqrt{n} \left| \left( \frac{\hat{F}_1^{-1}(p) - F_1^{-1}(p)}{\hat{\sigma}_{\mathcal{H}_0}} \right) - \left( \frac{\hat{F}_2^{-1}(p) - F_2^{-1}(p)}{\hat{\sigma}_{\mathcal{H}_0}} \right) + \frac{\Delta}{\hat{\sigma}_{\mathcal{H}_0}} \right| > q_{1-\alpha/2} \right) \\ &\approx P_{\mathcal{H}_1} \left( \frac{\sqrt{n}}{\hat{\sigma}_{\mathcal{H}_0}} \left( \frac{\hat{F}_1(F_1^{-1}(p)) - p}{f_1(F_1^{-1}(p))} - \frac{\hat{F}_2(F_2^{-1}(p)) - p}{f_2(F_2^{-1}(p))} \right) > q_{1-\alpha/2} - \frac{\sqrt{n}\Delta}{\hat{\sigma}_{\mathcal{H}_0}} \right) \\ &\quad + P_{\mathcal{H}_1} \left( \frac{\sqrt{n}}{\hat{\sigma}_{\mathcal{H}_0}} \left( \frac{\hat{F}_1(F_1^{-1}(p)) - p}{f_1(F_1^{-1}(p))} - \frac{\hat{F}_2(F_2^{-1}(p)) - p}{f_2(F_2^{-1}(p))} \right) < -q_{1-\alpha/2} - \frac{\sqrt{n}\Delta}{\hat{\sigma}_{\mathcal{H}_0}} \right) \\ &\approx P_{\mathcal{H}_1} \left( \frac{Z_n}{\hat{\sigma}_{\mathcal{H}_0}} > q_{1-\alpha/2} - \frac{\sqrt{n}\Delta}{\hat{\sigma}_{\mathcal{H}_0}} \right) + P_{\mathcal{H}_1} \left( \frac{Z_n}{\hat{\sigma}_{\mathcal{H}_0}} < -q_{1-\alpha/2} - \frac{\sqrt{n}\Delta}{\hat{\sigma}_{\mathcal{H}_0}} \right), \end{aligned}$$

where the expression in the fourth equality comes from Lemma 1 from Kosorok<sup>1</sup>. We conclude from the convergence of  $Z_n/\hat{\sigma}_{\mathcal{H}_0}$  towards a centered Gaussian random variable.

## 1.2 Multivariate test

In this section, we present the proofs for the results in Section 2.2 of the main document, for the multivariate test.

**Result 4.** For  $k = 1, 2$ ,

$$\sqrt{n} \begin{bmatrix} \frac{\hat{F}_k^{-1}(p_1) - F_k^{-1}(p_1)}{f_k(F_k^{-1}(p_1))} \\ \vdots \\ \frac{\hat{F}_k^{-1}(p_J) - F_k^{-1}(p_J)}{f_k(F_k^{-1}(p_J))} \end{bmatrix} \xrightarrow{d} \mathcal{N}(0, \Upsilon_{F_k}) \text{ as } n \rightarrow \infty,$$

where:

$$(\Upsilon_{F_k})_{jl} = \begin{cases} \frac{(1 - p_j)^2 \int_0^{F_k^{-1}(p_j)} \frac{d\Lambda_k(x)}{H_k(x)}}{\mu_k(f_k(F_k^{-1}(p_j)))^2}, & \text{if } j = l \\ \frac{(1 - p_j)(1 - p_l) \int_0^{F_k^{-1}(p_j) \wedge F_k^{-1}(p_l)} \frac{d\Lambda_k(x)}{H_k(x)}}{\mu_k f_k(F_k^{-1}(p_j)) f_k(F_k^{-1}(p_l))}, & \text{otherwise.} \end{cases}$$

**Proof.** From Lemma 1 in Kosorok<sup>1</sup>, we have:

$$\begin{bmatrix} \hat{F}_k^{-1}(p_1) - F_k^{-1}(p_1) \\ \vdots \\ \hat{F}_k^{-1}(p_J) - F_k^{-1}(p_J) \end{bmatrix} = U_k + o_p(1/\sqrt{n_k}),$$

where

$$U_k = \begin{bmatrix} \frac{\hat{F}_k(F_k^{-1}(p_1)) - p_1}{f_k(F_k^{-1}(p_1))} \\ \vdots \\ \frac{\hat{F}_k(F_k^{-1}(p_J)) - p_J}{f_k(F_k^{-1}(p_J))} \end{bmatrix}.$$

From Theorem 6.3.1 from Fleming and Harrington<sup>2</sup>,  $\sqrt{n_k}U_k$  converges to a centered multivariate Gaussian random variable where its variance matrix has entries  $(j, l)$  equal to:

$$\frac{(1 - p_j)(1 - p_l) \int_0^{F_k^{-1}(p_j) \wedge F_k^{-1}(p_l)} \frac{d\Lambda_k(x)}{H_k(x)}}{f_k(F_k^{-1}(p_j)) f_k(F_k^{-1}(p_l))}.$$

The result follows since  $n_k/n \rightarrow \mu_k$  as  $n \rightarrow \infty$ .

**Result 5.** Under  $\mathcal{H}_0 : F_1^{-1}(p_j) = F_2^{-1}(p_j), j = 1, \dots, J$ ,

$$\mathcal{Z}_n = \sqrt{n} \begin{bmatrix} \hat{F}_1^{-1}(p_1) - \hat{F}_2^{-1}(p_1) \\ \vdots \\ \hat{F}_1^{-1}(p_J) - \hat{F}_2^{-1}(p_J) \end{bmatrix} \xrightarrow{d} \mathcal{N}(0, \Psi) \text{ as } n \rightarrow \infty,$$

where  $\Psi = \Upsilon_{F_1} + \Upsilon_{F_2}$ .

The test statistic, expressed as  $\mathfrak{T}_n = \mathcal{Z}_n^T \Psi^{-1} \mathcal{Z}_n$ , converges in distribution towards a  $\chi_J^2$  as  $n \rightarrow \infty$  under  $\mathcal{H}_0$ .

**Proof.** Since the two treatment groups are independent, we have under  $\mathcal{H}_0$

$$\sqrt{n} \begin{bmatrix} \hat{F}_1^{-1}(p_1) - \hat{F}_2^{-1}(p_1) \\ \vdots \\ \hat{F}_1^{-1}(p_J) - \hat{F}_2^{-1}(p_J) \end{bmatrix} = \sqrt{n} \begin{bmatrix} \frac{\hat{F}_1^{-1}(p_1) - F_1^{-1}(p_1)}{f_1(F_1^{-1}(p_1))} \\ \vdots \\ \frac{\hat{F}_1^{-1}(p_J) - F_1^{-1}(p_J)}{f_1(F_1^{-1}(p_J))} \end{bmatrix} - \sqrt{n} \begin{bmatrix} \frac{\hat{F}_2^{-1}(p_1) - F_2^{-1}(p_1)}{f_2(F_2^{-1}(p_1))} \\ \vdots \\ \frac{\hat{F}_2^{-1}(p_J) - F_2^{-1}(p_J)}{f_2(F_2^{-1}(p_J))} \end{bmatrix} + o_p(1/\sqrt{n}).$$

From Result 4,

$$\mathcal{Z}_n = \sqrt{n} \begin{bmatrix} \hat{F}_1^{-1}(p_1) - \hat{F}_2^{-1}(p_1) \\ \vdots \\ \hat{F}_1^{-1}(p_J) - \hat{F}_2^{-1}(p_J) \end{bmatrix} \xrightarrow{d} \mathcal{N}(0, \Psi),$$

where  $\Psi = \Upsilon_{F_1} + \Upsilon_{F_2}$ . From these results, we conclude that, under  $\mathcal{H}_0$ ,  $\mathfrak{T}_n \xrightarrow{d} \chi_J^2$  as  $n \rightarrow \infty$ .

**Result 6.** Under  $\mathcal{H}_1 : F_1^{-1}(p_j) - F_2^{-1}(p_j) = \Delta_j, j = 1, \dots, J$ ,  $\mathfrak{T}_n$  is asymptotically equivalent to  $\chi_J^2(\Psi^{-1/2}\xi)$ , an uncentered chi-squared distribution with  $J$  degrees of freedom and mean  $\Psi^{-1/2}\xi$ , with

$$\xi = \sqrt{n} \begin{bmatrix} \Delta_1 \\ \vdots \\ \Delta_J \end{bmatrix}.$$

We then have the following asymptotic formula for the power of the test of level  $\alpha$ :

$$1 - \beta = F_{\chi_J^2(\Psi^{-1/2}\xi)}(q_{J,1-\alpha}),$$

denoting as  $F_{\chi_J^2(\Psi^{-1/2}\xi)}$  the cumulative distribution function of this chi-squared distribution and  $q_{J,1-\alpha}$  as the quantile of order  $1 - \alpha$  of the chi-squared distribution with  $J$  degrees of freedom.

**Proof.** We denote:

$$Y_n = \sqrt{n} \begin{bmatrix} \hat{F}_1^{-1}(p_1) - F_1^{-1}(p_1) \\ \vdots \\ \hat{F}_1^{-1}(p_J) - F_1^{-1}(p_J) \end{bmatrix} - \sqrt{n} \begin{bmatrix} \hat{F}_2^{-1}(p_1) - F_2^{-1}(p_1) \\ \vdots \\ \hat{F}_2^{-1}(p_J) - F_2^{-1}(p_J) \end{bmatrix}.$$

Under  $\mathcal{H}_1$ , we write:

$$\mathcal{Z}_n = Y_n + \xi.$$

From Lemma 1 in Kosorok<sup>1</sup>, we have:

$$Y_n = \sqrt{n} \begin{bmatrix} \frac{\hat{F}_1(F_1^{-1}(p_1)) - p_1}{f_1(F_1^{-1}(p_1))} \\ \vdots \\ \frac{\hat{F}_1(F_1^{-1}(p_J)) - p_J}{f_1(F_1^{-1}(p_J))} \end{bmatrix} - \sqrt{n} \begin{bmatrix} \frac{\hat{F}_2(F_2^{-1}(p_1)) - p_1}{f_2(F_2^{-1}(p_1))} \\ \vdots \\ \frac{\hat{F}_2(F_2^{-1}(p_J)) - p_J}{f_2(F_2^{-1}(p_J))} \end{bmatrix} + o_p(1/\sqrt{n}).$$

The first and second term on the right-hand side of this equation converge in distribution respectively to  $\mathcal{N}(0, \Upsilon_{F_1})$  and  $\mathcal{N}(0, \Upsilon_{F_2})$  as  $n \rightarrow \infty$ . Therefore,

$$Y_n \xrightarrow{d} \mathcal{N}(0, \Psi), \text{ as } n \rightarrow \infty,$$

and  $\mathcal{Z}_n$  is asymptotically equivalent to a  $\mathcal{N}(\xi, \Psi)$ . From the consistency of  $\hat{\Psi}$ ,  $\mathcal{Z}_n^T \hat{\Psi}^{-1} \mathcal{Z}_n$  is asymptotically equivalent to  $\chi_J^2(\Psi^{-1/2}\xi)$ . We conclude from the definition of the power,

$$\begin{aligned} 1 - \beta &= P_{\mathcal{H}_1}(\mathfrak{T}_n > q_{J,1-\alpha}) \\ &\approx F_{\chi_J^2(\Psi^{-1/2}\xi)}(q_{J,1-\alpha}). \end{aligned}$$

## 2 Details on the estimation of the density

In the main document, two different methods are proposed for the estimation of  $f_k(F_k^{-1}(p))$ ,  $k = 1, 2$ : a resampling procedure based on the method from Lin *et al.*<sup>3</sup> and a kernel density estimator. The first method only estimates the densities at one point, the quantile  $F_k^{-1}(p)$ , while the second method estimates the whole function  $f_k(t)$  from which the estimator at the quantile is obtained by setting  $t = F_k^{-1}(p)$ . In Section 2.1 the resampling procedure is explained, while details for the kernel density estimator are provided in Section 2.2.

### 2.1 Resampling procedure

We propose a resampling procedure that allows to estimate  $f(F^{-1}(p))$  the density at a given quantile, for a given probability  $0 < p < 1$ . We present a method inspired by Lin *et al.*<sup>3</sup> in order to perform such task in a resampling procedure. We require the densities at the quantiles to be strictly positive, and we

denote as  $\hat{F}$  the consistent estimator for  $F$  obtained from the usual Kaplan-Meier estimation. Taking this estimator we obtain  $\hat{F}^{-1}(p)$  the estimators of the inverse distribution at  $p$ . Then we propose the following resampling procedure:

1. Generate  $B$  realizations of the Gaussian  $\varepsilon \sim \mathcal{N}(0, \sigma^2)$ , denoted by  $\varepsilon_1, \dots, \varepsilon_B$
2. Calculate  $\sqrt{n} \left( \hat{F} \left( \hat{F}^{-1}(p) + \frac{\varepsilon_b}{\sqrt{n}} \right) - p \right)$ ,  $b = 1, \dots, B$  and denote them as  $y_b$ , then the least squares estimate of  $f(F^{-1}(p))$  is  $\hat{A} = (x'x)^{-1}x'Y$ , where  $x = (\varepsilon_1, \dots, \varepsilon_B)^T$  and  $Y = (y_1, \dots, y_B)^T$

We advocate that the variance of the Gaussian variables must be carefully chosen as it may impact the quality of estimation of the density. To illustrate this phenomenon, we study the behavior of the Mean Squared Error (MSE) when the sample size and  $\sigma$  change. Based on those results, we propose a grid-search method to automatically choose an optimal value for  $\sigma$ .

In Figure 1, we illustrate the MSE for a range of values of  $\sigma$  when estimating the median of an exponential distribution with rate 1.5. The true value of the density at the median is 0.75 and censoring follows an exponential distribution with rate 0.12. We generate  $B = 10000$  Gaussians and we replicate the code 100 times.

We notice that, for small sample sizes, the value of  $\sigma^2$  plays an important role in the value of the MSE. Indeed, as one increases sample size, the region where MSE is minimized becomes broader, which allows for greater flexibility when choosing the variance within a wider interval of values where the MSE is small. Consequently, variance selection is particularly important when working with small sample sizes. For all sample sizes, we observe that the MSE decreases until it reaches a plateau, where it remains low over a range of  $\sigma$  values, before increasing again. Our goal is then to select a value of  $\sigma$  that lays in such interval, which grows broader as sample size increases.

To identify this plateau, we estimate the density at the quantile over a grid of  $\sigma$  values and examine the results in small neighborhoods. We look for an interval where the estimated density shows the smallest local variation within its region, and select  $\sigma$  a value within this interval.

This procedure is illustrated for the estimation of the median of the exponential with rate 1.5, with exponential censoring with rate 0.12. We consider  $\sigma$  values ranging from 0 to 10 in increments of 0.05 and examine smaller neighborhoods, each containing 20 values for the estimated density at the median.

In Figure 2 we illustrate the estimation of the density at the median for each  $\sigma$ . The vertical line represents the selected  $\sigma$  by our procedure, which is equal to 3.65. We obtain an estimation of the density at the median equal to 0.72. In Figure 3, we illustrate the absolute difference between the estimated density at the median and the true value 0.75, for each  $\sigma$ . We see that our procedure selects a value of  $\sigma$  that lays inside the region where this difference is minimized.

Our method has been illustrated in the exponential framework, but the same reasoning can be applied to other distributions. The procedure has been implemented in R and all code is available in order to perform the variance selection automatically using the proposed grid-search algorithm, as well as the density estimation at a given quantile using the selected variance.

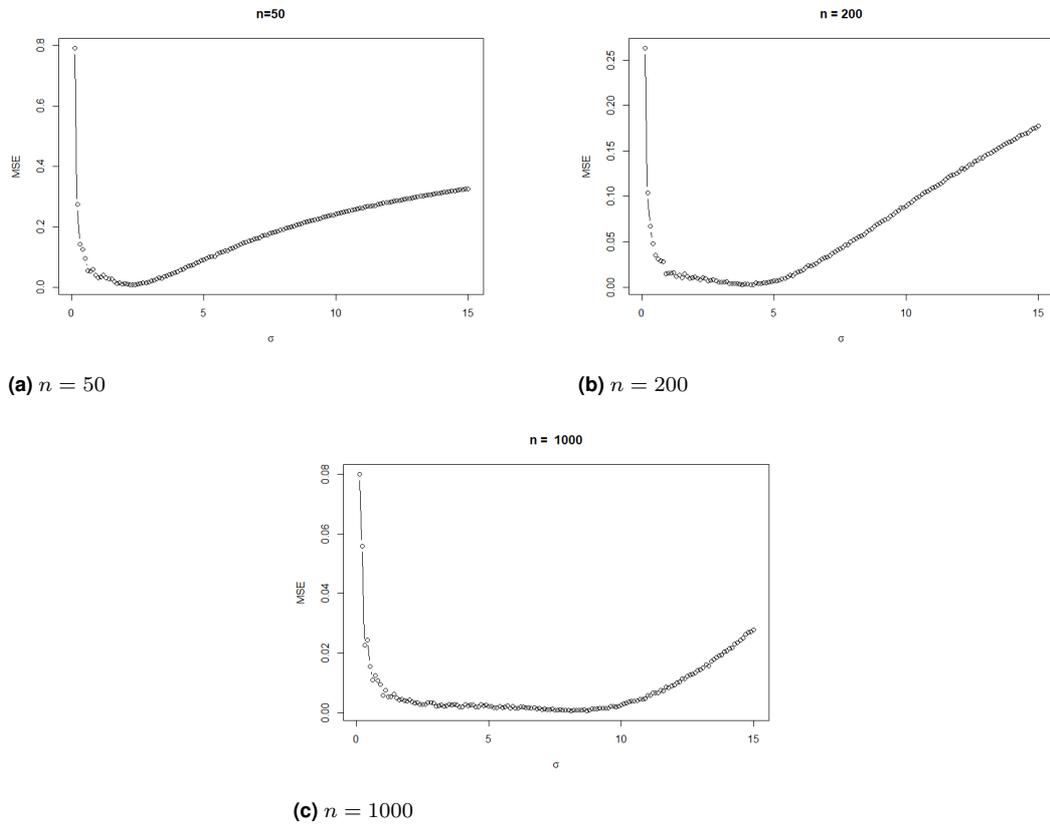

**Figure 1.** Comparison of MSE with respect to  $\sigma$  for different sample sizes.

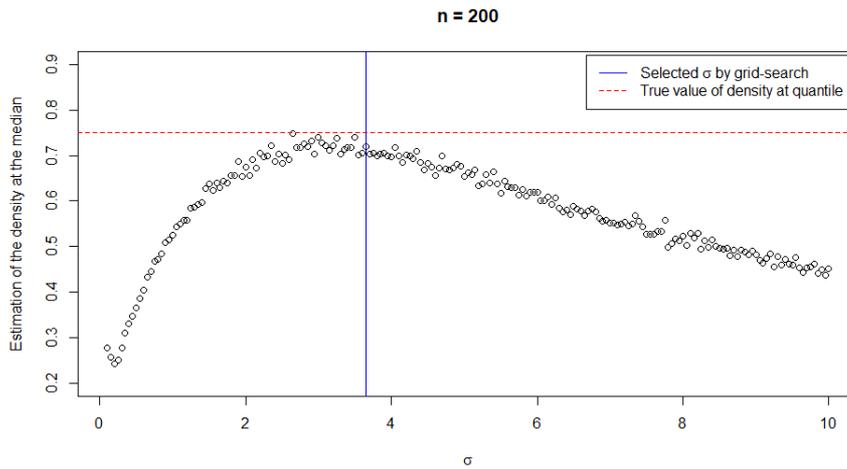

**Figure 2.** Example of density estimation at the median with respect to  $\sigma$ .

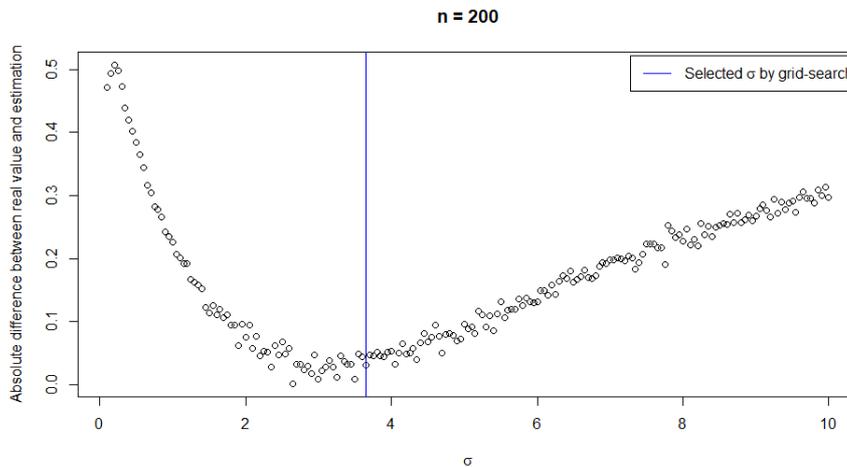

**Figure 3.** Absolute difference between the true density at median and its estimation by the proposed method, with respect to  $\sigma$ .

## 2.2 Kernel density estimation

In the presence of censoring, a typical kernel estimator of the density can be constructed by estimating the censoring distribution from the Kaplan-Meier estimator. In Földes *et al.*<sup>4</sup>, Diehl and Stute<sup>5</sup> the following estimator has been proposed:

$$\hat{f}_h(t) = \frac{1}{nh} \sum_{i=1}^n \frac{\delta_i}{\hat{S}_{\text{cens}}(T_i)} K\left(\frac{T_i - t}{h}\right),$$

where  $\hat{S}_{\text{cens}}$  is the Kaplan-Meier estimator of the censoring survival function and  $K$  a kernel satisfying standard conditions. In order to compute this estimator, the kernel and the bandwidth must be chosen. In our implementation, a Gaussian kernel was taken and the bandwidth was obtained from cross-validation. For the choice of the bandwidth, the goal of the method is to try to minimize the Integrated Squared Error (ISE), defined, for  $k = 1, 2$ , as:

$$\begin{aligned} \text{ISE}(\hat{f}_h) &= \int \left(\hat{f}_h(t) - f_k(t)\right)^2 dt \\ &= \int \hat{f}_h^2(t) dt - 2 \int \hat{f}_h(t) f_k(t) dt + \int f_k^2(t) dt. \end{aligned}$$

In this expression the last term does not depend on  $h$  and can be omitted. On the other hand, the term  $\int \hat{f}_h(t) f_k(t) dt$  is estimated by:

$$\hat{J}(h) = \frac{1}{n(n-1)h} \sum_{i \neq j} K\left(\frac{T_i - T_j}{h}\right) \frac{\delta_{ik} \delta_{jk}}{\hat{S}_{\text{cens}}(T_i) \hat{S}_{\text{cens}}(T_j)}.$$

Using the consistency of the Kaplan-Meier estimator, it can easily be shown that this estimator converges in probability, as  $n$  tends to infinity, towards  $\int \hat{f}_h(t) f_k(t) dt$  (see Marron and Padgett<sup>6</sup>). In conclusion, our cross-validated estimator is defined as the Gaussian kernel estimator with bandwidth chosen as the minimizer of  $\int \hat{f}_h^2(t) dt - 2\hat{J}(h)$ , that is:

$$\hat{h} = \arg \min_h \left\{ \int \hat{f}_h^2(t) dt - \frac{2}{n(n-1)h} \sum_{i \neq j} K\left(\frac{T_i - T_j}{h}\right) \frac{\delta_{ik} \delta_{jk}}{\hat{S}_{\text{cens}}(T_i) \hat{S}_{\text{cens}}(T_j)} \right\}.$$

We refer the reader to Marron and Padgett<sup>6</sup> for more details about the cross-validation bandwidth selector and theoretical results regarding its validity.

## References

1. Kosorok MR. Two-sample quantile tests under general conditions. *Biometrika*. 1999;86(4):909–21.
2. Fleming TR, Harrington DP. *Counting Processes and Survival Analysis*. New York: John Wiley & Sons; 1991.
3. Lin C, Zhang L, Zhou Y. Conditional quantile residual lifetime models for right censored data. *Lifetime Data Anal*. 2015;21:75–96.
4. Földes A, Rejtő L, Winter BB. Strong consistency properties of nonparametric estimators for randomly censored data, II: Estimation of density and failure rate. *Period Math Hungar*. 1981;12:15–29.
5. Diehl S, Stute W. Kernel density and hazard function estimation in the presence of censoring. *J Multivar Anal*. 1988;25(2):299–310.
6. Marron JS, Padgett WJ. Asymptotically optimal bandwidth selection for kernel density estimators from randomly right-censored samples. *Ann Stat*. 1987;15:1520–35.
